# Supplementary material for: Narrow-linewidth tin-vacancy centers in a diamond waveguide
Source: arXiv:2005.10385 ancillary file (2020-07-28)
Supplement: Supplementary file 1 [file SI.pdf]

# Supporting Information for Narrow-linewidth tin-vacancy centers in a diamond waveguide

Alison E. Rugar,[*,†,#] Constantin Dory,[†,#] Shahriar Aghaeimeibodi,[†,#] Haiyu Lu,[‡,¶] Shuo Sun,[†] Sattwik Deb Mishra,[†] Zhi-Xun Shen,[‡,§,¶,‖] Nicholas A. Melosh,[‖,⊥,¶] and Jelena Vučković[†]

†*E. L. Ginzton Laboratory, Stanford University, Stanford, CA 94305, USA*

‡*Department of Physics, Stanford University, Stanford, California 94305, United States*

¶*Geballe Laboratory for Advanced Materials, Stanford University, Stanford, California 94305, United States*

§*Department of Applied Physics, Stanford University, Stanford, California 94305, United States*

‖*Stanford Institute for Materials and Energy Sciences, SLAC National Accelerator Laboratory, Menlo Park, California 94025, United States*

⊥*Department of Materials Science and Engineering, Stanford University, Stanford, California 94305, United States*

#*These authors contributed equally to this work.*

E-mail: arugar@stanford.edu

## Additional photoluminescence measurements

We fabricated more than 1000 waveguide structures on a 2 × 2 mm$^2$ diamond chip. We inspected 12 waveguides in the center of the chip where we expect the fabrication and the SIIG method to perform most reliably. We confirmed the presence of the SnV$^-$ centers in

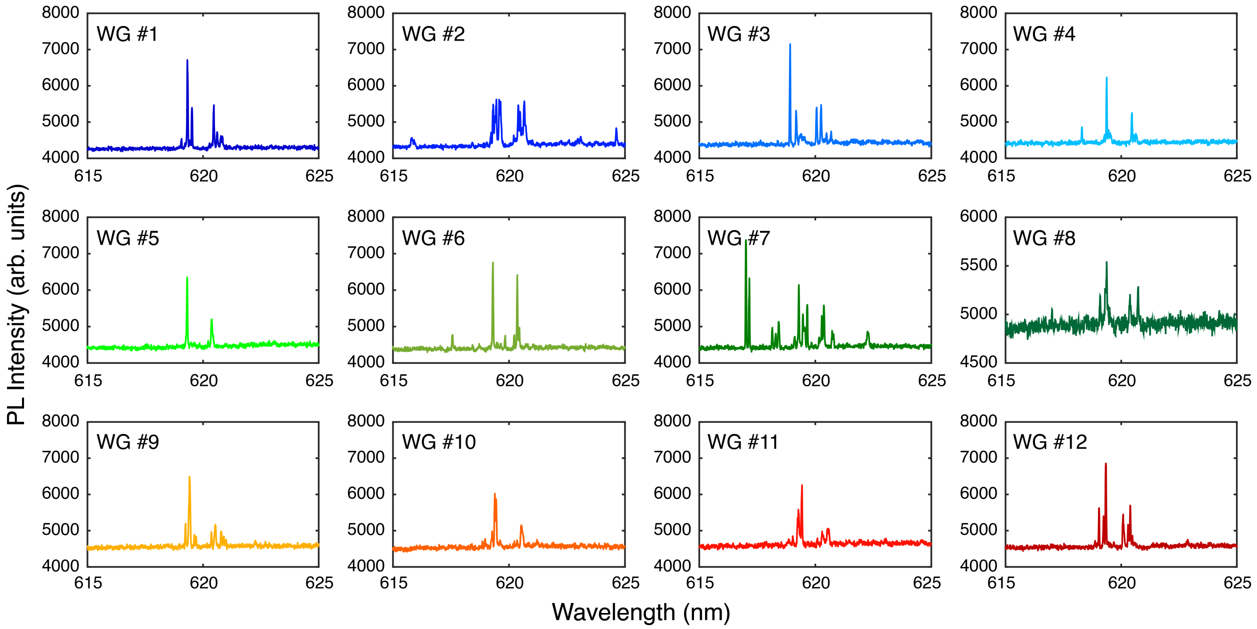


Figure S1: PL spectra collected on 12 waveguides (WG) with excitation and collection (MM fiber) aligned on the same spot.

these waveguides by measuring the PL spectra in the top-down configuration, as we did in Figure 2(b) of the main text. The spectra in Figure S1 show that all the inspected waveguide structures contained at least one $SnV^-$ center.

# Linewidths

Through PLE, we measured the linewidths of several $SnV^-$ centers in addition to the two presented in Figure 3 of the main text. In Figure S2, we present four more sets of PLE data from different $SnV^-$ centers. The data in Figures S2(a) and (b) were acquired in the VC-to-VC configuration, with 60 nW excitation. The data in Figures S2(c) and (d) were acquired in the top-down configuration, with 4-nW and 5.5-nW excitation respectively. The six Lorentzians that we fit to the data presented in Figure S2 have linewidths of $32 \pm 3$, $24 \pm 11$, $75 \pm 9$, $28 \pm 4$, $29 \pm 1$, and $25 \pm 5$ MHz, yielding an average linewidth of $36 \pm 3$ MHz.

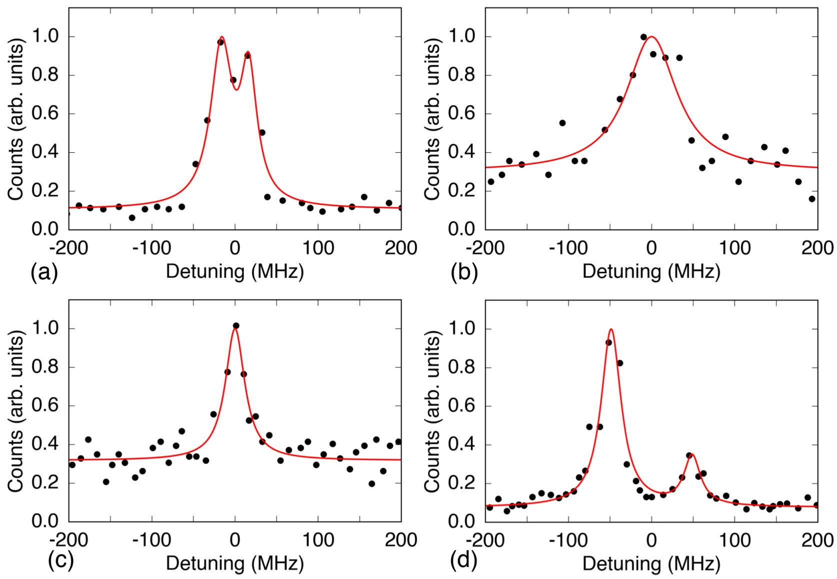


Figure S2: Linewidths of additional $SnV^-$ centers in diamond waveguides. Data are in black, and Lorentzian fits are red. (a) PLE dataset 1, acquired in the VC-to-VC configuration with 60-nW excitation power. Lower energy peak has a linewidth of $32 \pm 3$ MHz and the higher energy peak has a linewidth of $24 \pm 11$ MHz. (b) PLE dataset 2, acquired in VC-to-VC with 60-nW excitation power. Linewidth is $75 \pm 9$ MHz. (c) PLE dataset 3, acquired in the top-down configuration with 4-nW excitation power. Linewidth is $28 \pm 4$ MHz. (d) PLE dataset 4, acquired in the top-down configuration with 5.5-nW excitation power. Lower energy peak has a linewidth of $29 \pm 1$ MHz and the higher energy peak has a linewidth of $25 \pm 5$ MHz.

# Blinking

We define the occurrence of blinking to be a laser scan in which a PLE resonance was not detected. Starting with PLE data that was collected for ten minutes ($full\_data$), we separate the consecutive laser scans. To determine if the emitter blinked in a specific scan ($single\_scan$), we compare the maximum value of the scan to the sum of the mean and twice the standard deviation of all the data from the ten-minute acquisition. In other words, if $max(single\_scan) \leq \langle full\_data \rangle + 2\sigma_{full\_data}$, the emitter is considered to have blinked in that scan. Using this definition of blinking, we studied the dependence of blinking on excitation power and how many $SnV^-$ centers in waveguides blink during PLE.

Figure S3(a)-(d) show the PLE data collected for ten minutes each with excitation powers of 15, 30, 60, and 140 nW, respectively. Consecutive scans are offset vertically for clarity.

The scans in which the emitter blinked are marked in red. The fraction of collected scans in which the emitter blinked is plotted as a function of excitation power in Figure S3(e). The point for 140-nW excitation is pink because the color center stopped emitting after several passes through resonance, which is a special case of blinking.

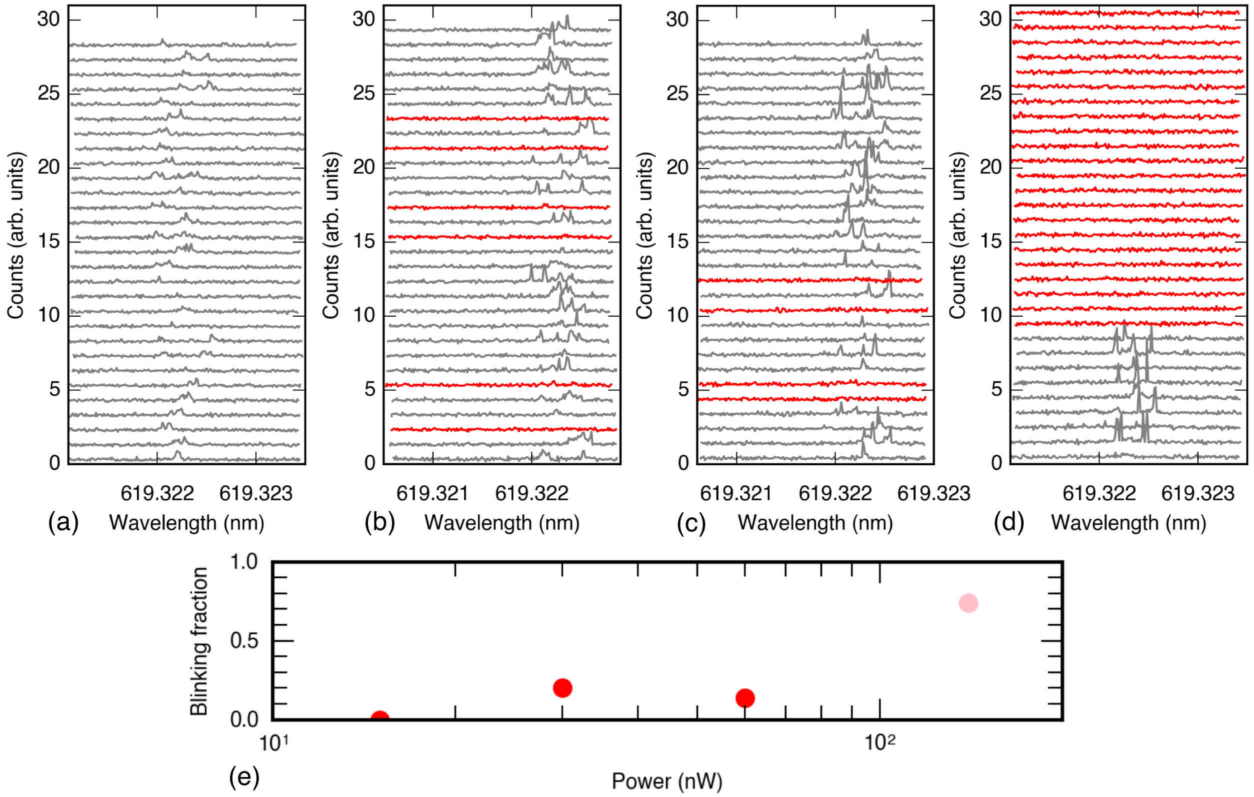


Figure S3: Blinking of $SnV^-$ centers in waveguides. PLE data from laser scans repeated for ten minutes at excitation powers of (a) 15 nW, (b) 30 nW, (c) 60 nW, and (d) 140 nW. Scans in which the $SnV^-$ center blinked are plotted in red. (e) Fraction of scans in which blinking was detected plotted against excitation power. The data point at 140 nW is pink because the $SnV^-$ ceased to emit a PLE signal after the first several scans.

We found that when a $SnV^-$ center stops emitting, 532-nm excitation can turn the $SnV^-$ center back "on," as shown in Figure S4. Consecutive PLE scans are offset vertically for clarity, starting with the first scan at the bottom of the plot. The emitter blinked in two consecutive PLE scans, plotted in red in Figure S4. In the following scan, plotted in green, the emitter blinked for a third time. At the end of this scan, a 532-nm laser was unblocked for $\sim 3$ seconds. The green illumination excited many emitters in the vicinity, resulting in

elevated counts for the duration of the green pulse. All the scans acquired after the green pulse displayed PLE signal.

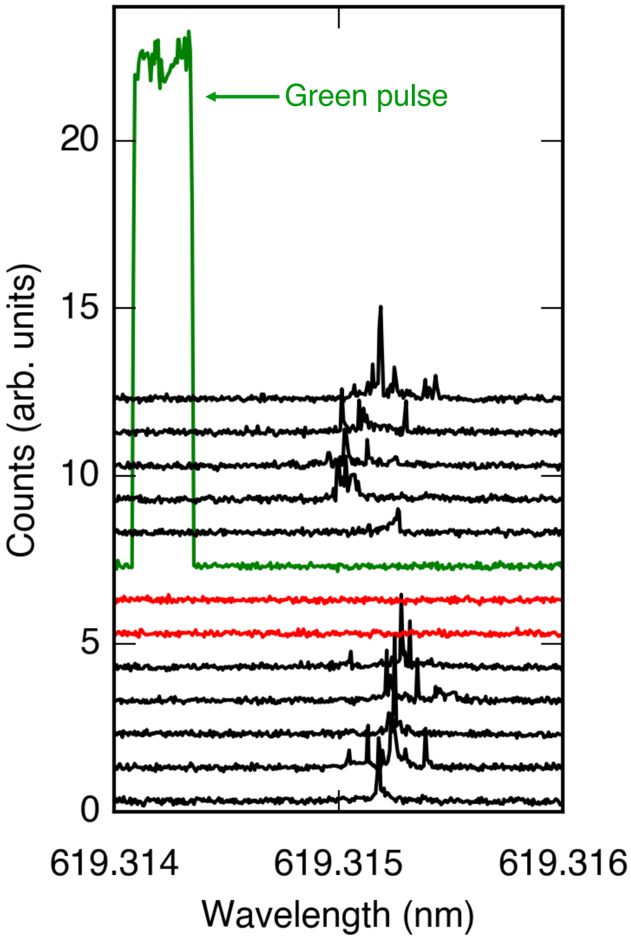


Figure S4: $SnV^-$ center emission recovered with pulse of green. Consecutive PLE scans are offset vertically for clarity, starting with the first scan at the bottom of the plot. The emitter blinked in two consecutive scans, plotted in red. The 532-nm excitation was then unblocked for $\sim 3$ seconds during the scan plotted in green. Counts were elevated for the duration of the green pulse. The scan with the green pulse was excluded from calculations to find the occurrences of blinking.

To determine how many emitters blink, we surveyed nine different $SnV^-$ centers in waveguides. We collected PLE data for ten minutes as we did for the power-dependence measurement described previously. Seven out of nine $SnV^-$ centers studied blinked at least once during the ten-minute PLE measurements.

# Spectral diffusion

To further investigate spectral diffusion, we repeated the PLE measurement of Figures 4(b) and 4(c) of the main text for ten distinct emitters in five waveguides. Figure S5(a) is a scatter plot representing spectral diffusion and center wavelength of the C transitions of the studied $SnV^-$ centers. Two emitters marked by the red arrow showed particularly stable emission, and their time trace is plotted in the Figure 4(b) of the main text. The average spectral diffusion of the ten emitters studied is 240.3 MHz.

We analyzed the effect of laser power on spectral diffusion of the emitter marked by the blue arrow in Figure S5(a). We varied the power between 5 nW and 140 nW. These limits are set by the vanishing signal-to-noise ratio of the PLE measurement at low powers and high blinking probability at high powers. Figure S5(b) shows that to the extent of our measurement error, the excitation power within the acceptable range does not significantly affect the diffusion.

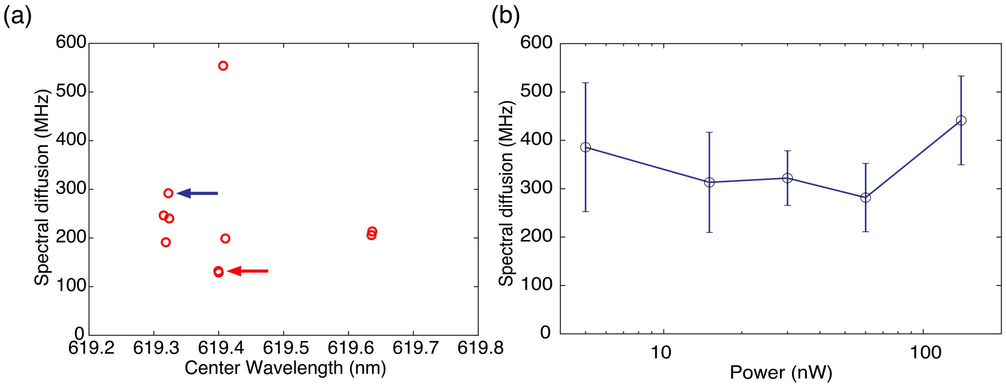


Figure S5: Spectral diffusion of $SnV^-$ centers in waveguides. (a) Scatter plot of spectral diffusion and center wavelength of ten $SnV^-$ centers. Two emitters marked by the red arrow are represented in Figures 4(b) and 4(c) of the main text. (b) Spectral diffusion measurement at different laser powers. We used the $SnV^-$ center marked by the blue arrow in (a).
